# Supplementary material for: The GANfather: Controllable generation of malicious activity to improve defence systems
Source: arXiv:2307.13787 source file (2023-07-25)
Supplement: Supplementary file 1 [file appendix.tex]

\setcounter{table}{0}

\setcounter{figure}{0}

\section{Appendix}
%Ablation studies: D; rules; objective; categorical sampling.
%Techniques to increase variety.
%Different pooling operations.
%Closeness to real data: trade-off between being close to real and moving money.
%Can include other generators that were not the best.

\subsection{Extended Methods}

\begin{table}[H]
    \centering
    \begin{tabular}{c|c|c}
        Index & Layer & Output shape\\
        \hline
        0 & Linear(100, 400) & (400,)\\
        1 & Linear(400, 1600) & (1600,)\\
        2 & Linear(1600, 5000) & (5000,)\\
          & Reshape & (5,10,10,10)\\
        3 & ConvTranspose1d(10,10,4,2,1) & (5,10,20,10)\\
        4 & ConvTranspose1d(10,10,4,2,1) & (5,10,40,10)\\
        5 & ConvTranspose1d(10,10,4,2,1) & (5,10,80,10)\\
        6 & ConvTranspose1d(10,10,4,2,1) & (5,10,160,10)\\
          & Split amounts and probabilities & (5,10,160,10)\\
        7 & ConvTranspose1d(10,10,4,2,1) & (5,10,320,10)\\
        8 & Conv1d(10,1,1,1,0) & (5,10,320)\\
          & Categorical sampling & (5,10,320)
    \end{tabular}
    \caption{AML generator architecture.}
    \label{tab:03_aml_genarch}
\end{table}

\begin{table}[h]
    \centering
    \begin{tabular}{c|c|c}
        Index & Layer & Output shape\\
        \hline
        0 & Conv1d(1,10,6,4,1) & (5,10,80,10)\\
        1 & Conv1d(10,10,6,4,1) & (5,10,20,10)\\
        2 & Conv1d(10,5,6,4,1) & (5,10,5,5)\\
          & Reshape & (5,2,5,25)\\
          & Mean pooling & (1,2,1,25)\\
          & Concatenate amounts and probabilities & (100,)\\
        3 & Linear(100,128) & (128,)\\
        4 & Linear(128,32) & (32,)\\
        5 & Linear(32,1) & (1,)
    \end{tabular}
    \caption{AML discriminator architecture.}
    \label{tab:03_aml_disarch}
\end{table}

\begin{table}[h]
    \centering
    \begin{tabular}{l|l}
        $\alpha$ & $1$ \\
        $\beta$  & $[10^2, 10^5]$ \\
        $\gamma$ & $[10^3, 4\times10^3]$ \\
        learning rate    & $[10^{-4}, 3\times10^{-3}]$
    \end{tabular}
    \caption{Hyperparameter search space on the AML use case.}
    \label{tab:03_aml_hpsp}
\end{table}

%\subsubsection{Experimental details: Recommender Systems}

\begin{table}[h]
    \centering
    \begin{tabular}{c|c|c}
        Index & Layer & Output shape\\
        \hline
        0 & ResBlock(128,128) & (128,)\\
        1 & ResBlock(128,128) & (128,)\\
          & Split ratings and probabilities & (128,)\\
        2 & ResBlock(128,128) & (128,)\\
        3 & ResBlock(128,64) & (64,)\\
        4 & Linear(64,3706) & (3706,)\\
          & Categorical sampling & (3706,)
    \end{tabular}
    \caption{RS generator architecture.}
    \label{tab:03_rs_genarch}
\end{table}

\begin{table}[h]
    \centering
    \begin{tabular}{c|c|c}
        Index & Layer & Output shape\\
        \hline
        0 & Dense(3706,64) & (64,)\\
        1 & ResBlock(64,128) & (128,)\\
        2 & ResBlock(128,64) & (64,)\\
          & Concatenate ratings and probabilities & (128,)\\
        3 & ResBlock(128,128) & (128,)\\
        4 & ResBlock(128,128) & (128,)\\
        5 & Linear(128,1) & (1,)
    \end{tabular}
    \caption{RS discriminator architecture.}
    \label{tab:03_rs_disarch}
\end{table}

\begin{table}[h]
    \centering
    \begin{tabular}{l|l}
        $\alpha$ & $[10^{-5}, 1]$ \\
        learning rate & $[10^{-5}, 3\times10^{-4}]$
    \end{tabular}
    \caption{Hyperparameter search space on the RS use case.}
    \label{tab:03_rs_hpsp}
\end{table}
